# Supplementary material for: Bridging the Gap: Studio-like Avatar Creation from a Monocular Phone Capture
Source: arXiv:2407.19593 source file (2024-07-30)
Supplement: Supplementary file 2 [file 12_appendix.tex]

\section{Texture and Render Results}
\begin{figure*}[h!]
    \centering
    \includegraphics[width=0.95\linewidth]{suppmat-figs/All-Tex-Suppmat-400ppi.pdf}
    
    \caption{\small{\textbf{Comparisons on Unpaired Phone-Captured Data}: In comparison to prior work, our method excels in generating texture maps with superior preservation of identity, enhanced photorealism in facial details, more uniform illumination, and improved inpainting of missing regions.
    }}
    \label{fig:all_tex}
\end{figure*}
In \fig{all_tex}, we show more qualitative results of the texture maps generated with our method versus prior art. As can be seen, across all subjects, our method generates texture maps that have better quality illumination, facial details and inpainting of missing regions. In Figs 2-10, we show multiview renders of these subjects (and a few more) using the Universal Prior Model from AVA \cite{cao2022authentic}. Again, we see that the avatars generated using the texture maps from our method are significantly more photorealistic than prior art.  
\input{Suppmat-render-figs}
\section{Ablation of optimization resolution}
\begin{table}[h]
\begin{center}
\small
\scalebox{0.85}{
\begin{tabular}{lcccr}
\toprule
  \midrule
  Models  & Full Network opt & Opt8 (Ours)  & Opt16    \\
\midrule
 FaceID \(\downarrow\) & \(5.01e-4\) &  \(\mathcolorbox{yellow}{4.31e-4}\) & \(\mathcolorbox{pink}{4.30e-4}\) \\
 \midrule
 KID \(\downarrow\) &  \(\mathcolorbox{pink}{1.36e-3}\) &  \(\mathcolorbox{yellow}{1.42e-3}\) & \(1.63e-3\) \\
\bottomrule
\end{tabular}}
\caption{\small{Ablation of optimization resolution.  \mathcolorbox{pink}{\text{Best}} and \mathcolorbox{Yellow}{\text{Second Best}} scores are highlighted. } }

\label{tab:opt_aba}
\vspace{-0.5cm}
\end{center}
\end{table}

As described in Section 3.1 of the paper, we optimize \(\GMug\) using the following loss:
\begin{smequation}
\underset{\GMug^{\theta(8+)}}{\text{min}} \underset{\mathcal{D}_{Studio}}{\text{max}}\mathcal{L}_{Adv} +  \mathcal{L}_{R1} + \mathcal{L}_{Percp-Recons} +\lambda_{1}\mathcal{L}_{Percp} + \lambda_{2}\mathcal{L}_{FaceID}
\label{eq:opt}
\end{smequation}
where \(\GMug^{\theta(8+)}\) denotes optimizing the parameters of the generator after the \(8\times 8 \) resolution. The intuition behind this is that identity-specific information is stored in the low-resolution maps and freezing the parameters of the lower resolution boosts identity preservation. In \tab{opt_aba}, we ablate this intuition. We compare optimizing the full network (`Full Network Opt'), optimizing after the \(8\times 8\) resolution and optimizing after the \(16\times 16\) resolution (`Opt16'). To measure identity preservation we use the FaceID metric and to measure the fidelity to the target distribution we use the Kernel Inception Distance (KID) \cite{StyleGANADA} metric. As can be seen, optimizing after the \(8\times 8 \) resolution gives us the best balance between identity preservation and fidelity to the target distribution. Optimizing the whole network (`Full Network Opt') yields a better KID but at the cost of a significantly worse identity preservation (a higher FaceID). On the flip side, optimizing after the \(16\times 16\) (`Opt16') results is a marginal improvement in FaceID but significantly worse KID.  
\section{Ablation of \(\mathcal{L}_{FaceID}\) and  \(\mathcal{L}_{Percp}\)}
In this section, we ablate \(\mathcal{L}_{FaceID} \text{ and } \mathcal{L}_{Percp} \) from \eq{opt}. As can be seen in \fig{faceID_LPIPS_aba} and \tab{faceid_lpips_aba}, not using \(\mathcal{L}_{FaceID} \text{ and } \mathcal{L}_{Percp} \) severely degrades performance and leads to non-convergent results. Using \(\mathcal{L}_{Percp}\), leads to significant improvements in training stability and results but there is still an identity shift. Using both \(\mathcal{L}_{FaceID} \text{ and } \mathcal{L}_{Percp} \) yields the best results with the identity strongly preserved after the transfer to studio-like lighting and inpainting of the missing regions.
\begin{table}[h]
\begin{center}
\small
\scalebox{0.85}{
\begin{tabular}{l{c}p{2cm}{c}p{2.5cm}{c}p{3.5cm}}
\toprule
  \midrule
  Models  & Full Loss & w/o \(\mathcal{L}_{FaceID}\)  & w/o \(\mathcal{L}_{FaceID}\) and  \(\mathcal{L}_{Percp}\)    \\
\midrule
 FaceID \(\downarrow\) & \(\mathcolorbox{pink}{5.36e-4}\) &  \(\mathcolorbox{yellow}{1.33e-3}\) & \(2.79e-3\) \\
\bottomrule
\end{tabular}}
\caption{\small{Ablation of Losses.  \mathcolorbox{pink}{\text{Best}} and \mathcolorbox{Yellow}{\text{Second Best}} scores are highlighted.  Note: These are the results of \(\GMug\) without the facial details added by our diffusion model } }

\label{tab:faceid_lpips_aba}
\vspace{-0.5cm}
\end{center}
\end{table}

\begin{figure*}[h!]
    \centering
    \includegraphics[width=0.95\linewidth]{suppmat-figs/FaceIDLPIPS-Aba.pdf}
    
    \caption{\small{\textbf{Ablation of FaceID and LPIPS loss}: As can be seen, not using \(\mathcal{L}_{FaceID} \text{ and } \mathcal{L}_{Percp} \) leads to a serve deterioration in performance. Not using \(\mathcal{L}_{FaceID}\) causes a significant identity shift. Using the full loss leads to the best results. Note: These are the results of \(\GMug\) without the facial details added by our diffusion model. 
    }}
    \label{fig:faceID_LPIPS_aba}
\end{figure*}
\section{Ablation of \(\mathcal{L}_{Percp-Recons}\)}
In this section, we ablate \(\mathcal{L}_{Percp-Recons}\) from \eq{opt}. While \(\mathcal{L}_{FaceID} \text{ and } \mathcal{L}_{Percp} \) help preserve identity and lead to more stable training, they're do not penalize global skin-tone shifts that may occur when an in-the-wild texture map is transferred to studio-like lighting as can be seen in \fig{LPIPS_recons_aba}. Using \(\mathcal{L}_{Percp-Recons}\) with a very small amount of data helps prevent this as it forces \(\GMug\) to maintain skin-tone while transferring from in-the-wild lighting to studio-like lighting. 
\begin{figure*}[h!]
    \centering
    \includegraphics[width=0.95\linewidth]{suppmat-figs/LPIPS_Recons_aba.pdf}
    
    \caption{\small{\textbf{Ablation of  \(\mathcal{L}_{Percp-Recons}\)}: Not using \(\mathcal{L}_{Percp-Recons}\) leads to a minor shift in skin-tone. 
    }}
    \label{fig:LPIPS_recons_aba}
\end{figure*}
\section{Limitations}
As mentioned in the paper, our method only models the head, important regions such as the shoulder and torso and not modelled and are left for future work. Additionally, as shown in \fig{fail}, our method cannot handle head accessories well, this is because the studio-captured data does not have any head-accessories.
\begin{figure*}[h!]
    \centering
    \includegraphics[width=0.95\linewidth]{suppmat-figs/Fail.png}
    
    \caption{\small{\textbf{Limitations}: Our method fails to preserve head-accessories
    }}
    \label{fig:fail}
\end{figure*}
